# Supplementary material for: Nanophotonic quantum storage at telecommunications wavelength
Source: arXiv:1904.08052 ancillary file (2019-04-17)
Supplement: Supplementary file 1 [file Craiciu_2019_Nanophotonic_quantum_storage_SM.pdf]

# Supplementary Materials

## Nanophotonic quantum storage at telecommunications wavelength

Ioana Craiciu,<sup>1,2</sup> Mi Lei,<sup>1,2</sup> Jake Rochman,<sup>1,2</sup> Jonathan M.  
Kindem,<sup>1,2</sup> John G. Bartholomew,<sup>1,2</sup> Evan Miyazono,<sup>1,2</sup>  
Tian Zhong,<sup>1,2,\*</sup> Neil Sinclair,<sup>3,4</sup> and Andrei Faraon<sup>1,2,†</sup>

<sup>1</sup>*Kavli Nanoscience Institute and Thomas J. Watson,  
Sr., Laboratory of Applied Physics,  
California Institute of Technology, Pasadena, California 91125, USA*

<sup>2</sup>*Institute for Quantum Information and Matter,  
California Institute of Technology, Pasadena, California 91125, USA*

<sup>3</sup>*Division of Physics, Mathematics and Astronomy,  
California Institute of Technology, Pasadena, CA 91125, USA*

<sup>4</sup>*Alliance for Quantum Technologies,  
California Institute of Technology, Pasadena, CA 91125, USA*

(Dated: April 16, 2019)

---

\* Currently at: Institute of Molecular Engineering, University of Chicago, Chicago, Illinois 60637, USA

† Corresponding author: faraon@caltech.edu

## I. EXPERIMENTAL DETAILS

A fiber-coupled tunable external-cavity diode laser was used to probe the nanobeam device and implement the AFC storage protocol. One percent of the laser light was directed to a wavemeter for measurement. Another one percent of the laser light was picked off and sent to a locking setup, in which the laser frequency was stabilized by locking to a home-built fiber cavity using the Pound-Drever-Hall technique [1]. The rest of the light was directed through two acousto-optical modulators (AOMs) for pulse shaping. An electro-optic phase modulator (EOM) was used to generate strong sidebands necessary for initialization (see Section IV). The EOM was also used to add a  $\pi$  phase shift to pulses as required for fidelity measurements (see Section VIII). Neutral density (ND) filters and polarization paddles provided attenuation and polarization control, respectively. A circulator directed light to the  $^{167}\text{Er}^{3+}:\text{YSO}$  crystal located inside a dilution refrigerator. The sample was mounted using indium solder onto a copper plate, which was thermally contacted to the 25 mK stage of a dilution refrigerator. A stack of  $xyz$  nanopositioners under the plate was used to optimize free space coupling. An aspheric lens pair focused light from a fiber onto the angled coupler of the resonator. Light from the sample was directed through the circulator onto a superconducting nanowire single photon detector (SNSPD) at  $\sim 100$  mK. A micro electro-mechanical switch prevented strong initialization and comb creation pulses from reaching the SNSPD. A magnetic field  $\mathbf{B} = 380$  mT was applied to the sample using two cylindrical permanent magnets for all measurements.

## II. SPECTRAL INITIALIZATION AND HYPERFINE $T_1$ IN BULK $^{167}\text{Er}^{3+}:\text{YSO}$

The hyperfine lifetime ( $T_1$ ) of  $^{167}\text{Er}^{3+}$  ions in YSO was measured using spectrally resolved optical pumping in an applied field of 380 mT parallel to the  $D_1$  crystal axis, and a nominal temperature of 25 mK. SM Figure 1a shows a schematic of the  $^{167}\text{Er}^{3+}:\text{YSO}$  energy levels. With a splitting of 80 GHz at 25 mK, the electron spin is frozen ( $\hbar\omega \ll k_B T$ ).

SM Figure 1b shows a scan of the inhomogeneously broadened  $^{167}\text{Er}^{3+}:\text{YSO}$  absorption line (black curve) in a bulk crystal. Transitions between individual hyperfine levels (in the lower electron spin branch) in the optical ground and excited state manifolds are partially resolved. A wide spectral transparency (trench) was created in this absorption line by

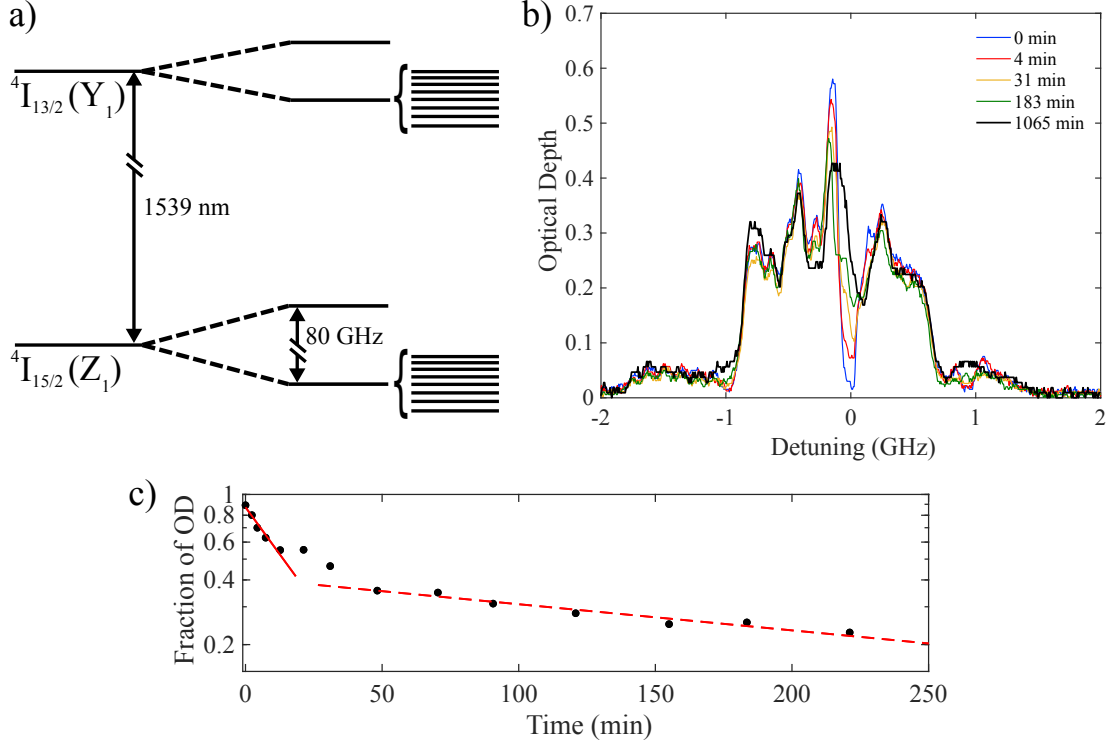

SM Figure 1. a) Schematic of energy levels of  $^{167}\text{Er}^{3+}:\text{YSO}$  with an applied field of 380 mT parallel to the  $D_1$  crystal axis. For crystallographic site 2, the  $^4I_{15/2} \rightarrow ^4I_{13/2}$  transition between the lowest crystal field levels corresponds to a wavelength of 1539 nm [2]. Each of these levels ( $Z_1$  and  $Y_1$ ) is an electron spin doublet that, which the applied magnetic field splits by 80 GHz [3]. The  $I = 7/2$  nuclear spin of  $^{167}\text{Er}^{3+}$  splits each electron spin level into 8. The bottom 8 levels of both the ground and excited manifolds are shown. These are the levels participating in the optical transitions studied in this work. b) Inhomogeneous  $^{167}\text{Er}^{3+}:\text{YSO}$  line showing the hyperfine structure and a spectral trench at 0 GHz detuning, shown as a function of time after trench creation. The detuning is measured from  $194814 \text{ GHz} \pm 1 \text{ GHz}$ . c) Depth of trench as a fraction of optical depth (OD) as a function of time after trench creation.

optical pumping: a laser was scanned slowly and repeatedly over a 140 MHz band, which depleted those hyperfine levels with resonant transitions. The population was then allowed to return to its equilibrium distribution while measuring transmission using a room temperature InGaAs photodiode. The last measured distribution among ground state hyperfine levels was not thermal, as the long relaxation times prevent timely thermalization and even scanning the inhomogeneous line redistributes population. Scanning the line to probe the hole depth

likely led to an underestimation of  $T_1$  by redistributing population, but this effect was minimized by using low scan power.

The width of the trench was chosen to minimize effects of spectral diffusion on the  $T_1$  measurement. The depth of the spectral feature, or hole depth  $d$ , is a measure of how much population was pumped away from the hyperfine levels that were optically addressed:

$$d(t) = \frac{\text{optical depth}(t \rightarrow \infty) - \text{optical depth}(t)}{\text{optical depth}(t \rightarrow \infty)}. \quad (1)$$

The maximum  $d(t)$  achieved here was 0.9. This was partly limited by the large trench width, which was likely spanning multiple hyperfine transitions, leading to some pumping of population as the laser is swept to create the trench. Using smaller trenches, holes with depth of  $\sim 0.93$  were measured, where it became difficult to accurately measure the depth of the hole due to a noisy background from detector noise and Fabry-Perot resonances in the setup. It is also possible that hole depth is limited by the  $^{167}\text{Er}^{3+}$  isotopic purity.

SM Figure 1c shows the decay in time of the hole depth  $d(t)$  as measured in the center of the trench. The fast decay is fit to an exponential with a lifetime of 29 min, while the slow decay is fit to a lifetime of 6 hours. Following Reference [4], we interpret these lifetimes as a two-step change in the spectrum: first the trench fills in due to spin-spin interactions between  $^{167}\text{Er}^{3+}$  ions, then, at a slower rate, the population is redistributed among hyperfine levels due to spin-lattice interactions.

### III. DEVICE TEMPERATURE

Because of poor thermal conduction at low temperatures in insulating materials such as YSO, and the small cross section of the nanobeam, the device was warmer than its  $\sim 25$  mK surroundings whenever optical pulses were coupled in. The device temperature was estimated via the electron spin temperature, which was computed from the ratio between the lower and upper electron spin populations in the optical ground manifold using:

$$\frac{N_{|\uparrow\rangle}}{N_{|\downarrow\rangle}} = e^{-\frac{\hbar\omega}{k_B T}}. \quad (2)$$

Under an applied field of 380 mT, the electron spin in the optical ground state was frozen for any temperature under  $\sim 500$  mK. This is what enabled the long hyperfine lifetimes necessary for the main results of this work. To be sensitive to lower temperatures,

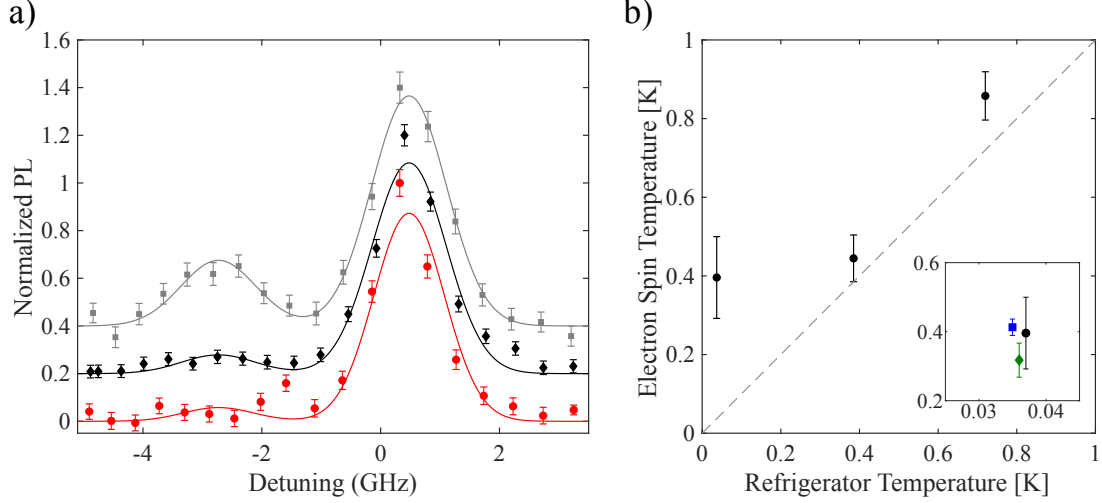

SM Figure 2. a) Photoluminescence from the nanobeam device as a function of detuning for three refrigerator temperatures: 720 mK (gray squares), 385 mK (black diamonds), 37 mK (red circles). Detuning is measured from  $194810 \pm 0.1$  GHz. The PL was collected after a  $500 \mu\text{s}$  resonant pulse at 0.3 pW (estimated power in nanobeam). Background counts were subtracted, and each curve was normalized and offset for clarity. Solid lines are fits to a sum of two Gaussians with equal widths and center frequencies 3.2 GHz apart. The transition from the  $|\downarrow\rangle$  ground state is at the higher frequency. Error bars are  $\sqrt{N_{\text{counts}}}$  for photon statistics. b) Electron spin temperatures computed from the PL data in (a), as a function of refrigerator temperature. Dashed gray line indicates where the two temperatures are equal. The inset shows a closeup of the 37 mK data point (black circle) and the electron spin temperatures estimated during the  $T_2$  measurement (green diamond) and the 165 ns storage experiment (blue square). To estimate the latter two temperatures, the same pattern of laser pulses as in the actual experiments was sent to the nanobeam, at 0.3 nW and 0.02 nW, respectively, and PL was collected after the pulses. Error bars are propagated  $\sqrt{N_{\text{counts}}}$  errors. In all measurements the laser frequency was slowly modulated within each transition to prevent hyperfine holeburning.

the electron spin population measurements were performed with a lower magnetic field of 110 mT (parallel to the  $D_1$  axis of the crystal), leading to an electron Zeeman splitting of  $\omega = 2\pi \times 23$  GHz, where the upper electron spin had detectable population down to  $\sim 250$  mK. Because the Zeeman splitting was still considerably greater than the hyperfine splitting, one can consider two electron spin states,  $|\downarrow\rangle$  and  $|\uparrow\rangle$ , each split into eight by the hyperfine interaction. The population in the two electron spin levels was measured via the

electron-spin-preserving optical transitions from each level. The nanobeam was tuned such that these transitions were both resonant with the cavity, and photoluminescence (PL) was collected as a function of frequency, as shown in SM Fig. 2a.  $N_{|\uparrow\rangle}/N_{|\downarrow\rangle}$  was extracted from the area ratio of the two transitions. SM Figure 2b shows the electron spin temperatures computed from these ratios for different dilution fridge temperatures. The inset in Fig. 2b shows the electron spin temperature measured under input power conditions identical to two experiments:  $317 \text{ mK} \pm 49 \text{ mK}$  for the  $T_2$  measurement in the nanobeam in SM Fig. 4 and  $413 \text{ mK} \pm 24 \text{ mK}$  for the 165 ns storage experiment in Fig. 2 of the main text. Assuming the electron spin is in thermal equilibrium with the device, we therefore estimated the temperature of our device during experiments to be  $\sim 400 \text{ mK}$ .

#### IV. HYPERFINE INITIALIZATION – DISCUSSION AND BULK RESULTS

Due to the hyperfine splitting in both ground and excited state manifolds in  $^{167}\text{Er}^{3+}:\text{YSO}$ , the inhomogeneous linewidth is effectively broadened from its true value of  $\sim 150 \text{ MHz}$  to  $\sim 1.5 \text{ GHz}$ , decreasing the optical depth in the center of the line, relative to an isotope with zero nuclear spin. Moving population into fewer hyperfine states can increase this optical depth. At high magnetic fields, the entire optical ground state population can be initialized into one hyperfine state [4] by pumping on all  $\Delta m = +1$  or all  $\Delta m = -1$  transitions. At  $380 \text{ mT} \parallel D_1$ , only a partial initialization can be performed because the  $\Delta m = \pm 1$  transitions are not fully resolved from the  $\Delta m = 0$  transitions. SM Figure 3 shows the  $^{167}\text{Er}^{3+}:\text{YSO}$  1539 nm transition in a bulk crystal, both with and without initialization, always with a spectral comb created in the center. Initialization was performed by turning on strong sidebands of the EOM modulator, and sweeping their detuning over a range of  $\pm(0.37 \text{ GHz} - 0.82 \text{ GHz})$ . This was the full range of the voltage controlled oscillator used to sweep the sidebands. A pulse sequence schematic is shown in Fig. 2b of the main text. This procedure moved population from the higher and lower energy hyperfine states to the middle few hyperfine states. The optical depth was improved by a factor of  $\sim 3$  compared to the uninitialized case, both in the bulk case shown in SM Fig. 3, and in the nanobeam, shown in the inset of Fig. 3c in the main text. Sweeping one sideband to pump on only one side of the inhomogeneous line produced a similar enhancement in optical depth. Preliminary studies have indicated that changing the angle of the magnetic field can also lead to separation of

$\Delta m = \pm 1$  transitions from the  $\Delta m = 0$  transitions for fields as low as 1 T, which would enable efficient hyperfine initialization at moderate magnetic fields.

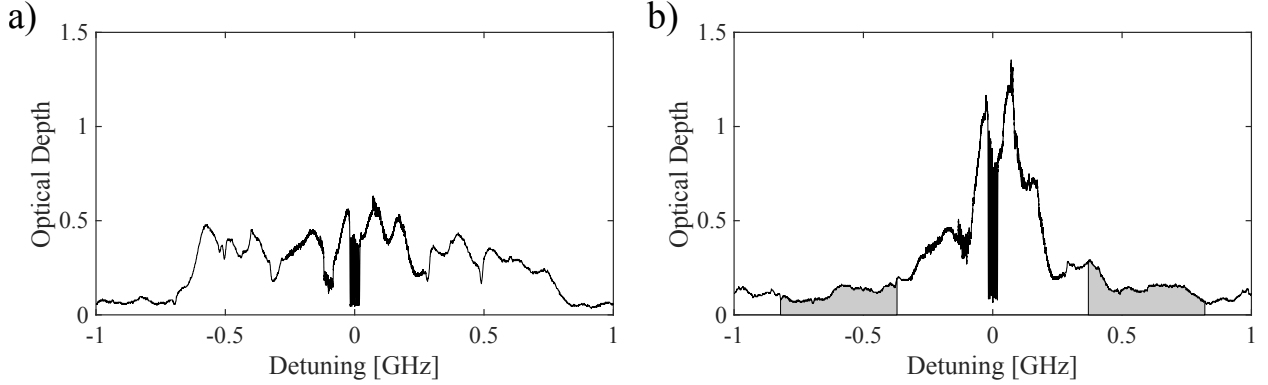

SM Figure 3. Absorption spectrum of the inhomogeneous line in bulk  $^{167}\text{Er}^{3+}:\text{YSO}$  at 18 mK and 380 mT (parallel to  $D_1$ ) with 40 MHz wide comb created in the center. a) Without initialization, peak optical depth of comb is 0.4. b) With initialization into few hyperfine states before comb creation, peak optical depth of comb is 0.9. Gray area shows the extent of the sweep of the EOM sidebands during the initialization step. The detuning was measured from  $194814 \text{ GHz} \pm 1 \text{ GHz}$ .

## V. FITTING THE CAVITY REFLECTION CURVE TO EXTRACT ENSEMBLE COOPERATIVITY

To extract the cooperativity of the coupling between the nanobeam resonator and the ensemble of  $^{167}\text{Er}^{3+}$  ions, we fit each cavity reflection spectrum shown in the inset of Figure 1c in the main text to

$$R = \alpha_1 \left| (1 - \alpha_f) + \alpha_f e^{i\theta_f} - \frac{i\kappa_{\text{coupling}}}{\omega - \omega_{\text{cavity}} + i\frac{\kappa}{2} + W(\omega, g_{\text{total}}, \Delta_{\text{ions}}, \omega_{\text{ions}})} \right|^2 + \alpha_2. \quad (3)$$

where  $\alpha_{1,2}$  are amplitude and background fit parameters,  $\alpha_f e^{i\theta_f}$  accounts for Fano interference (both  $\alpha_f$  and  $\theta_f$  are fit parameters),  $\kappa$  is the total cavity energy decay rate,  $\kappa_{\text{coupling}}$  is the coupling rate through the input/output port, and  $\omega_{\text{cavity}}$  is the cavity resonance frequency.  $\kappa = 27.3$  and  $\frac{\kappa_{\text{coupling}}}{\kappa} = 0.21$  were measured from reflectivity curves where the cavity was detuned from the  $^{167}\text{Er}^{3+}$  transition.  $W(\omega, g_{\text{total}}, \Delta_{\text{ions}}, \omega_{\text{ions}})$  is the absorption rate of the cavity field by the ensemble of ions,  $W \sim \sum_i \frac{g_i^2}{\omega - \omega_i}$ , where  $g_i$  is the coupling between one ion and the cavity [5, 6]. We approximate the irregular inhomogeneous/hyperfine line as a

Gaussian, and take from Reference [6] the expression for  $W$ :

$$W = i \frac{\sqrt{\pi \log 2} g_{\text{total}}^2}{\Delta_{\text{ions}}/2} \left[ 1 - \text{erfz} \left( -\frac{i \sqrt{\log 2} (\omega - \omega_{\text{ions}})}{\Delta_{\text{ions}}/2} \right) \right] \exp \left[ -\sqrt{\log 2} \left( \frac{\omega - \omega_{\text{ions}}}{\Delta_{\text{ions}}/2} \right)^2 \right], \quad (4)$$

where  $\Delta_{\text{ions}}$  is the linewidth of the ensemble transition,  $\omega_{\text{ions}}$  its the center,  $g_{\text{total}}^2 = \sum_i g_i^2$ . Finally, the ensemble cooperativity was computed using  $C = \frac{|W(\omega=\omega_{\text{ions}})|}{\kappa/2} = \frac{4\sqrt{\pi \log 2} g_{\text{total}}^2}{\kappa \Delta_{\text{ions}}}$  [7].

For the case with no initialization, the fit gave:  $\omega_{\text{cavity}} - \omega_{\text{ions}} = 2\pi \times 2.5$  GHz,  $g_{\text{total}} = 2\pi \times 0.79$  GHz,  $\Delta_{\text{ions}} = 2\pi \times 1.4$  GHz,  $C = 0.1$ .

For the case with initialization, the fit gave:  $\omega_{\text{cavity}} - \omega_{\text{ions}} = 2\pi \times 1.5$  GHz,  $g_{\text{total}} = 2\pi \times 0.70$  GHz,  $\Delta_{\text{ions}} = 2\pi \times 0.36$  GHz,  $C = 0.3$ .

## VI. COMPARISON OF THE OPTICAL $T_2$ TIME IN BULK AND IN THE NANOBEAM

By measuring two pulse photon echoes [8] as a function of time delay between pulses, the optical coherence time of ensembles of  $^{167}\text{Er}^{3+}:\text{YSO}$  ions was characterized in the center of the 1539 nm transition distribution, as shown in SM Figure 4. The laser was frequency stabilized by PDH locking to a home-built fiber cavity when measuring the bulk coherence at 35 mK ( $T_2 = 759 \mu\text{s}$ ). Without laser locking, this same curve had a double decay with a shorter exponential decay lifetime  $\sim 240 \mu\text{s}$ , which we interpret as being limited by laser frequency jitter. The coherence time of the ions coupled to the nanobeam cavity was  $149 \mu\text{s}$ , about 1/4 the coherence time of the bulk ions at the same dilution refrigerator temperature. This is due in part to the elevated temperature in the nanobeam compared to bulk. The nanobeam temperature was measured to be 317 mK (see Section III). The coherence time of the bulk ions at 1 K was found to have a similar value of  $136 \mu\text{s}$ . It is also possible that the fabrication of the nanobeam resonator caused disorder that affected the coherence time of the ions. Rare-earth ions coupled to similar nanobeam resonators have been shown to have coherence times similar to the bulk [9, 10], however, the longer bulk coherence times measured in the current work allow a much more sensitive probe of the ions' environment.

## VII. CREATING ATOMIC FREQUENCY COMBS

Two different procedures were used to create the AFCs. For longer memory times, the frequency difference between the teeth of the comb must be smaller, so the teeth themselves

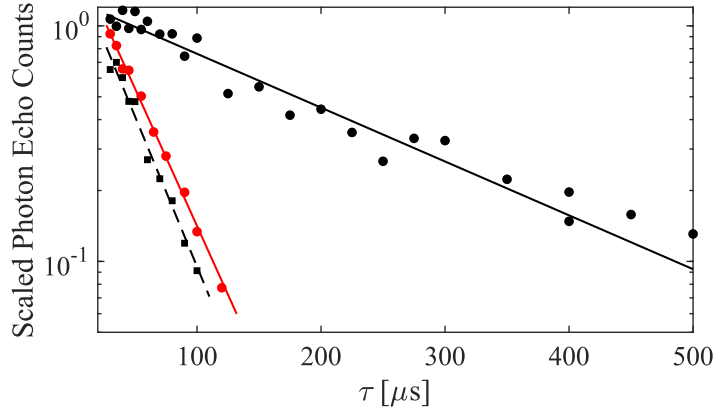

SM Figure 4. Two pulse photon echo amplitudes versus inter-pulse time delay with exponential fits; the vertical axis is scaled for clarity.  $T_2$  was measured to be  $4 \times \tau(1/e) = 759 \mu\text{s} \pm 41 \mu\text{s}$  in bulk at 35 mK (black circles and solid black line fit),  $136 \mu\text{s} \pm 9 \mu\text{s}$  in bulk at 940 mK (black squares and dashed black line fit), and  $149 \mu\text{s} \pm 4 \mu\text{s}$  in the nanobeam at 42 mK (red circles and solid red line fit). The above listed temperatures were measured at the dilution refrigerator stage to which the sample was thermally connected. The nanobeam temperature during  $T_2$  measurement was measured to be 317 mK (see Section III).

need also be narrower. Laser frequency jitter limits the minimum width of comb teeth, so longer storage times necessitate frequency stabilization of the laser. With the step-and-pump method, the laser must be stepped in frequency, and the method used to lock the laser (feeding back to the current) did not allow for both stepping and stabilizing the laser frequency. With the accumulated AFC method, no frequency modulation is required, so frequency stabilization was possible, enabling longer memory times. However, for short memory times, where laser jitter did not adversely affect the width of the teeth, the step-and-pump method led to a higher efficiency because the depth of the teeth across the comb was homogeneous (with accumulated AFC, the frequency comb has a sinc function envelope).

For the longest memory time of  $10 \mu\text{s}$ , the minimum spectral feature width of  $\sim 1 \text{ MHz}$  (limited by superhyperfine coupling) was larger than the comb tooth spacing of  $0.1 \text{ MHz}$ . The resulting atomic frequency comb was a convolution of the input frequency comb (the Fourier transform of the comb creation pulse pairs) with the minimum spectral feature of the ions. This lowered the contrast of the AFC: either ions were burned away from the maxima of the comb, decreasing  $\Gamma_{\text{comb}}$ , or ions were left in the minima of the comb, increasing  $\Gamma_{\text{bg}}$ ,

or both (see section IX). Any of these would decrease the memory efficiency (see Equation 12 in Section IX), and which scenario occurred would depend on the power and repetition number of the comb creation pulses. We chose the comb creation parameters by optimizing the efficiency of the memory (i.e. the amplitude of the output pulse).

### VIII. FIDELITY MEASUREMENT

In the absence of a single photon source, a lower bound on the storage fidelity of a single photon input state can be found using the decoy state analysis method [11, 12]. In this method, a time bin state  $\psi$  with a mean photon number  $\bar{n}$  is stored using the AFC protocol, and the fidelity  $F_\psi^{(\bar{n})}$  of storage is measured as

$$F_\psi^{(\bar{n})} = \frac{N_\psi}{N_\psi + N_{\phi \perp \psi}}, \quad (5)$$

where  $N_i (i = \psi, \phi)$  is the number of photons measured in the output time bin corresponding to  $\psi$ , and  $\phi \perp \psi$  denotes the state orthogonal to  $\psi$ . The gain of the output,  $Q_\psi^{(\bar{n})}$  is also estimated using,

$$Q_\psi^{(\bar{n})} = N_\psi + N_{\phi \perp \psi}. \quad (6)$$

$F_\psi^{(\bar{n})}$  and  $Q_\psi^{(\bar{n})}$  are measured for mean photon numbers  $\bar{n}_1$  and  $\bar{n}_2$ , where  $\bar{n}_1 < \bar{n}_2$ , and  $\bar{n}_2 < 1$ . The lower bound on the fidelity of storing a one-photon input state  $F_\psi^{(n=1,L)}$  is then computed using:

$$F_\psi^{(n=1,L)} = 1 - \frac{E_\psi^{(\bar{n}_1)} Q^{(\bar{n}_1)} \exp \bar{n}_1 - E^{(n=0)} Y^{(n=0)}}{Y^{(n=1,L)} \bar{n}_1}, \quad (7)$$

where

$$E_\psi^{(\bar{n})} = 1 - F_\psi^{(\bar{n})} \quad (8)$$

is the error rate of storing a state  $\psi$  with mean photon number  $\bar{n}$ , and

$$Y^{(n=1,L)} = \max \left[ Y^{(n=0)}, \frac{\bar{n}_2}{\bar{n}_2 \bar{n}_1 - \bar{n}_1^2} \left( Q^{(\bar{n}_1)} \exp \bar{n}_1 - Q^{(\bar{n}_2)} \exp \bar{n}_2 \frac{\bar{n}_1^2}{\bar{n}_2^2} - \frac{\bar{n}_2^2 - \bar{n}_1^2}{\bar{n}_2^2} Y^{(n=0)} \right) \right] \quad (9)$$

is the lower bound on the detection yield for the storage of a single photon state (see Reference [11]).  $Y^{(n=0)} = Q^{(n=0)}$  is the yield when the input state is vacuum, equal to the dark counts in all output time bins. The superscripts denote photon number, and whether the value is a lower bound ( $L$ ).  $E^{(n=0)}$  is the vacuum error rate, which is 0.5 by definition [11].

In order to obtain an average fidelity for all time bin states, the fidelities for storing time bin states  $|\text{early}\rangle$ ,  $|\text{late}\rangle$ ,  $|+\rangle = \frac{|\text{early}\rangle + |\text{late}\rangle}{\sqrt{2}}$  and  $|-\rangle = \frac{|\text{early}\rangle - |\text{late}\rangle}{\sqrt{2}}$  were measured for input photon numbers  $\bar{n} = 0.30$  and  $\bar{n} = 0.60$ . For input states  $|+\rangle$  and  $|-\rangle$ , an interferometer is required to measure  $N_\psi$  and  $N_{\phi\perp\psi}$ . Following Reference [13], a double atomic frequency comb was used as the interferometer, allowing for direct readout of  $F_+$  and  $F_-$ . The input pulses defining the  $|\text{early}\rangle$  and  $|\text{late}\rangle$  basis were 60 ns wide and 90 ns apart. A double AFC was used for measurements of all states, with the memory times associated with the two combs being  $t_1 = 210$  ns and  $t_2 = 300$  ns, such that  $t_1 - t_2 = 90$  ns. As SM Figure 5 shows, of the three output time bins, the first and third were used for measuring  $F_{\text{early}}$  and  $F_{\text{late}}$  while the second time bin was used for measuring  $F_+$  and  $F_-$ .

For computing the bound on the yield of a single photon in Equation 9,  $Q_-(Q_{\text{early}})$  and  $Q_+(Q_{\text{late}})$  were averaged to give  $Q_{+/-}$  ( $Q_{\text{early/late}}$ ), and the dark counts were averaged to give  $Y_{+/-}^{(n=0)}$  ( $Y_{\text{early/late}}^{(n=0)}$ ). From these, two different lower bounds on the single photon yield,  $Y_{+/-}^{(n=1,L)}$  and  $Y_{\text{early/late}}^{(n=1,L)}$  were computed. This was required because while the experiments to measure  $F_+$  and  $F_-$  were identical in every way except the input state, and the same holds for the experiments to measure  $F_{\text{early}}$  and  $F_{\text{late}}$ , the pairs of experiments differed from one another. For instance, because two output pulses overlapped to give a signal in measurements of  $F_+$  and  $F_-$ , the signal level was twice as large as for  $F_{\text{early}}$  and  $F_{\text{late}}$ , so the latter two experiments were conducted for twice as long to compensate.

Following Equation 7,  $F_+^{(n=1,L)}$  was therefore computed using:

$$F_+^{(n=1,L)} = 1 - \frac{E_+^{(\bar{n}_1)} Q_{+/-}^{(\bar{n}_1)} \exp \bar{n}_1 - E^{(n=0)} Y_{+/-}^{(n=0)}}{Y_{+/-}^{(n=1,L)} \bar{n}_1}, \quad (10)$$

with similar equations for the other three states.

The lower bound on the fidelity of storing an arbitrary single photon state was then computed as follows:

$$F_{\text{average}}^{(n=1,L)} = \frac{1}{3} \left( \frac{F_{\text{early}}^{(n=1,L)} + F_{\text{late}}^{(n=1,L)}}{2} \right) + \frac{2}{3} \left( \frac{F_+^{(n=1,L)} + F_-^{(n=1,L)}}{2} \right). \quad (11)$$

Table I summarizes the fidelity data used to compute  $F_{\text{average}}^{(n=1,L)} = 93.7\% \pm 2.4\%$ . The uncertainties are calculated based on  $\sqrt{N_{\text{photon}}}$  standard deviation on all  $N_\psi$  values due to Poissonian statistics of photon counting and the uncertainty, estimated to be 15%, of the

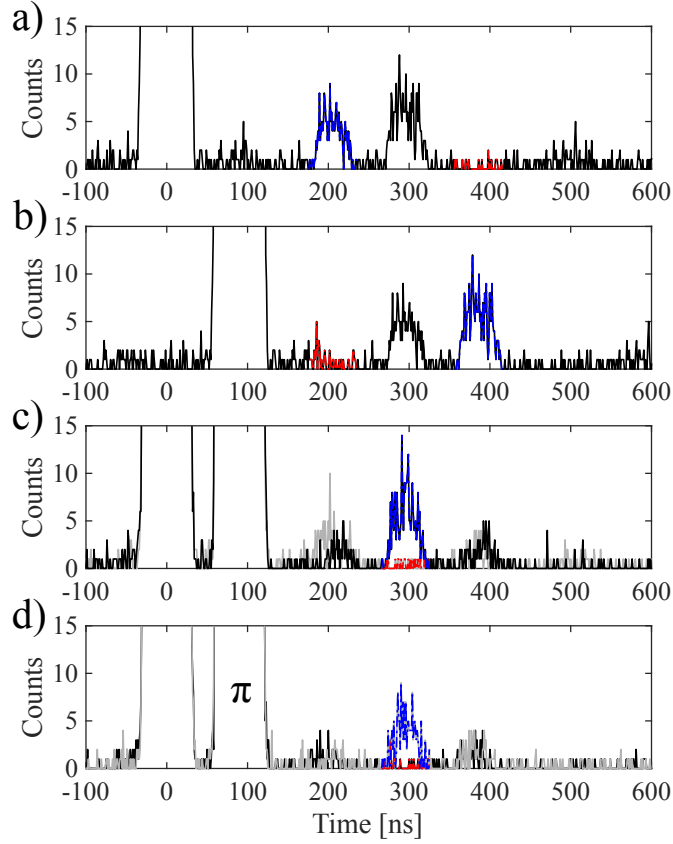

SM Figure 5. Part of the raw data used in the fidelity measurement.  $\bar{n} = 0.6$  input (left, cut off) and output pulses from double comb. Input pulses are time bin states a) early b) late, c) +, d) -. In all figures, blue (red) dash-dot line represents the 60 ns time bins counted as  $N_\psi$  ( $N_{\phi\perp\psi}$ ). Time resolution is 1 ns. The same data set, shown in a) and b), was used for both the early and late fidelity calculations, since absolute time is irrelevant. In this data set, a small pulse 100 ns after the read pulse can be seen. The origin of this pulse was unclear, but it disappeared in the absence of the double comb. In c) and d), the black curve represents data taken with comb detunings  $\delta_1 = \delta_2 = 0$ , while the gray curve represents data taken with  $\delta_1 = 0$ ,  $\delta_2 = \frac{\Delta_2}{2}$  ( $\phi_{\text{rel}} = \pi$ ).

mean input photon numbers,  $\bar{n}$ .

There were two main limits to the measured fidelity. The first was dark counts, which are uniformly distributed SNSPD detection events with an average rate of 18 Hz, believed to be caused by environmental photons at a wide range of wavelengths and electronic noise. The dark counts limited fidelity bound was estimated to be  $\sim 96.5\%$ . The remaining reduction

| Input photon number       | $\frac{1}{2} (F_{\text{early}} + F_{\text{late}})$                     | $\frac{1}{2} (F_+ + F_-)$                     |
|---------------------------|------------------------------------------------------------------------|-----------------------------------------------|
| $\bar{n} = 0.60 \pm 0.09$ | $89.04\% \pm 1.34\%$                                                   | $91.90\% \pm 1.32\%$                          |
| $\bar{n} = 0.30 \pm 0.05$ | $82.59\% \pm 1.80\%$                                                   | $90.75\% \pm 1.84\%$                          |
| $n = 0$                   | 50%                                                                    | 50%                                           |
|                           | $\frac{1}{2} (F_{\text{early}}^{(n=1,L)} + F_{\text{late}}^{(n=1,L)})$ | $\frac{1}{2} (F_+^{(n=1,L)} + F_-^{(n=1,L)})$ |
| $n = 1$                   | $89.85\% \pm 1.97\%$                                                   | $95.59\% \pm 3.37\%$                          |

TABLE I. Measured fidelities of storage in the nanobeam device.

in measured fidelity was caused by the double AFC being an imperfect interferometer. Specifically, we observed: (i) imperfect cancellation of the overlapped output pulses in the case of destructive interference, resulting from the different efficiencies of output pulses generated by the two spectral combs; (ii) a peak found at  $\sim 100$  ns that is an unexpected result of the double comb procedure, shown in SM Fig. 5b.

## IX. PREDICTED EFFICIENCY OF AFC STORAGE: CURRENT DEVICE AND FUTURE IMPROVEMENT

As described in References [5, 10, 14], the efficiency of an AFC memory in a resonator is given by:

$$\eta_{AFC} = \left( \frac{4\kappa_{\text{coupling}} \Gamma_{\text{comb}}}{(\kappa_{\text{total}} + \Gamma_{\text{comb}} + \Gamma_{\text{bg}})^2} \right)^2 \exp \left( -\frac{\pi^2}{2 \ln 2 (\Delta/\gamma)^2} \right). \quad (12)$$

The effective cooperativity  $C'$  of the atomic frequency comb is defined as:

$$C' \equiv \frac{\Gamma_{\text{comb}} + \Gamma_{\text{bg}}}{\kappa_{\text{total}}/2}, \quad (13)$$

where  $\Gamma_{\text{comb}}$  and  $\Gamma_{\text{bg}}$  are the absorption rates of the cavity field by the ensemble of ions in the comb and background, respectively. The background ions are the ions remaining after optical pumping, with transition frequencies where transparency is desired (i.e. between the teeth of the comb). Nonzero  $\Gamma_{\text{bg}}$  results from limitations in spectral holeburning, as discussed in Section II. Using  $\eta_{\text{spectral}}$ , the fractional optical depth of a spectral hole (in the language of Section II,  $\eta_{\text{spectral}} = d(t=0)$ ),  $\Delta$ , the inter-tooth spacing, and  $\gamma$ , the width of one comb tooth, these can be estimated as follows:

$$\Gamma_{\text{comb}} \approx \eta_{\text{spectral}} \frac{\gamma}{\Delta} \Gamma_{\text{ions}}, \quad (14)$$

$$\Gamma_{\text{bg}} = (1 - \eta_{\text{spectral}}) \Gamma_{\text{ions}}, \quad (15)$$

where

$$\begin{aligned} \eta_{\text{spectral}} &= \frac{N_{\text{ions}}(\text{comb peak}) - N_{\text{ions}}(\text{comb trough})}{N_{\text{ions}}(\text{comb peak})} \\ &= \frac{\text{initial optical depth} - \text{optical depth post initialization}}{\text{initial optical depth}} \end{aligned}$$

and  $\Gamma_{\text{ions}} = |W(\omega = \omega_{\text{ions}})| = \frac{\sqrt{\pi \log 2} g_{\text{total}}^2}{\Delta_{\text{ions}}/2}$  is the absorption rate of the cavity field by the ensemble of ions before comb preparation (see Section V). The effective cooperativity  $C'$  is therefore related to the cooperativity before the comb was created,  $C$  by  $C' = (\eta_{\text{spectral}} \frac{\gamma}{\Delta} + (1 - \eta_{\text{spectral}}))C$ . Rewriting the equation gives rise to the following expression for the memory efficiency of a real comb:

$$\eta_{\text{AFC}} = \left( \frac{1}{\frac{\Delta}{\gamma} \left( \frac{1}{\eta_{\text{spectral}}} - 1 \right) + 1} \frac{\kappa_{\text{coupling}}}{\kappa_{\text{total}}} \frac{4C'}{(1 + C')^2} \right)^2 \exp \left( -\frac{\pi^2}{2 \ln 2 (\Delta/\gamma)^2} \right). \quad (16)$$

The predicted efficiency for this device is  $\eta_{\text{AFC}} = 0.17\%$ , found using  $C = 0.3$ ,  $\frac{\kappa_{\text{coupling}}}{\kappa_{\text{total}}} = 0.21$ , a measured fidelity of  $\Delta/\gamma = 2.1$ , and by assuming a perfect comb  $\eta_{\text{spectral}} = 1$  (giving  $C' = 0.14$ ). This is similar to the measured value of  $0.20\%$  for a storage time of 165 ns.

To improve the memory efficiency, the two most important improvements that can be made are to increase the ensemble cooperativity, and to improve the ratio  $\frac{\kappa_{\text{coupling}}}{\kappa_{\text{total}}}$ . The first of these can be accomplished by increasing the doping of erbium in the YSO crystal ( $\times 4$  increase in  $C$  by increasing the ion concentration to 200 ppm, assuming no significant increase in inhomogeneous linewidth), and also by initializing into a single hyperfine state with 95% efficiency [4], before preparing a comb (an expected increase in  $C$  of approximately  $\times 2.5$ ). Using  $C = 3$  and  $\frac{\kappa_{\text{coupling}}}{\kappa_{\text{total}}} = 0.21$ , and a comb finesse of  $\Delta/\gamma = 3$ , ( $C' = 0.73$ ), the predicted efficiency is 3%.

At this point, the memory efficiency is mainly limited by the loss from the cavity. In the case of perfectly narrow, perfectly absorbing comb teeth with no background,  $C' \rightarrow 1$ ,  $\Delta/\gamma \rightarrow \infty$ ,  $\eta_{\text{spectral}} \rightarrow 1$ , the efficiency of the AFC becomes  $\left( \frac{\kappa_{\text{coupling}}}{\kappa_{\text{total}}} \right)^2 = \left( 1 - \frac{\kappa_{\text{intrinsic}} + \kappa_{\text{mirror 2}}}{\kappa_{\text{total}}} \right)^2$ . That is, in the limit of perfect spectral tailoring, the memory efficiency is limited by what fraction of the cavity decay rate is through the coupling port.

A memory efficiency greater than 90% can be achieved if the intrinsic quality factor of the resonator is increased from its current value of  $Q_i \sim 9000$  to 2 million, while increasing  $\frac{\kappa_{\text{coupling}}}{\kappa_{\text{total}}}$  to 0.97. The latter can be accomplished by making a resonator with one mirror having

a relatively lower reflectivity, and with minimal losses through other channels (transmission through second mirror, scattering, absorption). This calculation assumes the same material as described above (200 ppm, ideal initialization into one hyperfine state), and a comb finesse of  $\sim 13$ . It also accounts for a decrease by a factor of  $\sim 3$  in the cooperativity that results from switching to a hybrid silicon-YSO platform where the cavity-ion coupling is decreased because the optical mode couples evanescently to the ions. At this efficiency, the memory would match the performance of an optical fiber (0.15 dB/km) at  $t_{\text{storage}} = 10 \mu\text{s}$  [15].

For a finesse of 13 and a storage time of  $10 \mu\text{s}$ , the corresponding comb tooth width is  $\gamma = \frac{\Delta}{\text{finesse}} = 8 \text{ kHz}$ . This is too narrow for a material doped with Kramer’s ions such as  $^{167}\text{Er}^{3+}:\text{YSO}$ , where effective linewidths are limited by superhyperfine coupling to the host material’s nuclear spins. In  $\text{Er}^{3+}:\text{YSO}$ , superhyperfine broadening is of the order of 1 MHz [16, 17]. However, long memory times can still be achieved with a nanoresonator in this material by using the spin-wave AFC, where the stored coherence is transferred from the optical to the hyperfine manifold and back [18]. Coherence times of greater than 1 second have been measured for the hyperfine levels in  $^{167}\text{Er}^{3+}:\text{YSO}$  [4].

- 
- [1] R. W. P. Drever, J. L. Hall, F. V. Kowalski, J. Hough, G. M. Ford, A. J. Munley, and H. Ward, *Appl. Phys. B* **31**, 97 (1983).
  - [2] T. Böttger, Y. Sun, C. W. Thiel, and R. L. Cone, *Phys. Rev. B* **74**, 075107 (2006).
  - [3] Y. Sun, T. Böttger, C. W. Thiel, and R. L. Cone, *Phys. Rev. B* **77**, 085124 (2008).
  - [4] M. Rančić, M. P. Hedges, R. L. Ahlefeldt, and M. J. Sellars, *Nature Physics* **14**, 50 (2018).
  - [5] M. Afzelius and C. Simon, *Phys. Rev. A* **82**, 022310 (2010).
  - [6] I. Diniz, S. Portolan, R. Ferreira, J. M. Gérard, P. Bertet, and A. Auffèves, *Phys. Rev. A* **84**, 063810 (2011).
  - [7] E. Miyazono, I. Craiciu, A. Arbabi, T. Zhong, and A. Faraon, *Opt. Express* **25**, 2863 (2017).
  - [8] I. D. Abella, N. A. Kurnit, and S. R. Hartmann, *Phys. Rev.* **141**, 391 (1966).
  - [9] T. Zhong, J. M. Kindem, E. Miyazono, and A. Faraon, *Nature Communications* **6**, 8206 (2015).
  - [10] T. Zhong, J. M. Kindem, J. G. Bartholomew, J. Rochman, I. Craiciu, E. Miyazono, M. Bettinelli, E. Cavalli, V. Verma, S. W. Nam, F. Marsili, M. D. Shaw, A. D. Beyer, and A. Faraon,

- Science (2017), 10.1126/science.aan5959.
- [11] X. Ma, B. Qi, Y. Zhao, and H.-K. Lo, Phys. Rev. A **72**, 012326 (2005).
  - [12] N. Sinclair, E. Saglamyurek, H. Mallahzadeh, J. A. Slater, M. George, R. Ricken, M. P. Hedges, D. Oblak, C. Simon, W. Sohler, and W. Tittel, Phys. Rev. Lett. **113**, 053603 (2014).
  - [13] H. de Riedmatten, M. Afzelius, M. U. Staudt, C. Simon, and N. Gisin, Nature **456**, 773 (2008).
  - [14] S. A. Moiseev, S. N. Andrianov, and F. F. Gubaidullin, Phys. Rev. A **82**, 022311 (2010).
  - [15] Y.-W. Cho, G. T. Campbell, J. L. Everett, J. Bernu, D. B. Higginbottom, M. T. Cao, J. Geng, N. P. Robins, P. K. Lam, and B. C. Buchler, Optica **3**, 100 (2016).
  - [16] O. Guillot-Noël, H. Vezin, P. Goldner, F. Beaudoux, J. Vincent, J. Lejay, and I. Lorgeré, Phys. Rev. B **76**, 180408 (2007).
  - [17] B. Car, L. Veissier, A. Louchet-Chauvet, J.-L. Le Gouët, and T. Chanelière, Phys. Rev. Lett. **120**, 197401 (2018).
  - [18] M. Afzelius, C. Simon, H. de Riedmatten, and N. Gisin, Phys. Rev. A **79**, 052329 (2009).
